# Supplementary material for: Exploring Spatial Indexing for Accelerated Feature Retrieval in HPC
Source: arXiv:2106.13972 source file (2021-08-18)
Supplement: Supplementary file 1 [file libs-summary-appendix.tex]

\begin{table}[!htbp]
\caption{Additional information about the libraries evaluated in this paper}
\begin{tabular}{|l|l|l|l|l|}
\hline
\textbf{Library} &
  \textbf{\begin{tabular}[c]{@{}l@{}}Additional\\ Data structures\end{tabular}} &
  \textbf{\begin{tabular}[c]{@{}l@{}}Additional\\ Searches supported\end{tabular}} &
  \textbf{\begin{tabular}[c]{@{}l@{}}Static vs.\\ Dynamic\end{tabular}} &
  \textbf{Things to note} \\ \hline
\textbf{3DTK} &
  \textbf{\begin{tabular}[c]{@{}l@{}}octree\\ ANN k-d tree\\ANN BD tree\end{tabular}} &
  \textbf{\begin{tabular}[c]{@{}l@{}}k-d tree: KNN, KNN w. range;\\ Range (between two pts.)\\ octree: Nearest neighbor\end{tabular}} &
  \textbf{Static} &
  \textbf{} \\ \hline
\textbf{ALGLIB} &
  \textbf{} &
  \textbf{\begin{tabular}[c]{@{}l@{}}KNN, AKNN\\ Range (sphere)\end{tabular}} &
  \textbf{Static} &
  \textbf{} \\ \hline
\textbf{ANN} &
  \textbf{} &
  \textbf{\begin{tabular}[c]{@{}l@{}}W. or w/o radius:\\ KNN, Approximate KNN\end{tabular}} &
  \textbf{Static} &
  \textbf{\begin{tabular}[c]{@{}l@{}}Designed for high\\ dimensional data\end{tabular}} \\ \hline
\textbf{\begin{tabular}[c]{@{}l@{}}Boost\end{tabular}} &
  \textbf{} &
  \textbf{\begin{tabular}[c]{@{}l@{}}Intersects, overlap, etc.\\ for box or segment\\ KNN for point, box, segment\end{tabular}} &
  \textbf{\begin{tabular}[c]{@{}l@{}}Dynamic, self-balancing\\ Packing algorithm\end{tabular}} &
  \textbf{} \\ \hline
\textbf{CGAL} &
  \textbf{\begin{tabular}[c]{@{}l@{}}Other structures \\ for 2D searching\end{tabular}} &
  \textbf{\begin{tabular}[c]{@{}l@{}}k-d tree: exact and approximate:\\ KNN;\\ Furthest neighbor;\\ Range (sphere)\end{tabular}} &
  \textbf{\begin{tabular}[c]{@{}l@{}}K-d tree: dynamic,\\ not self balancing\\ Range trees: static\\ Segment tree: static \\ R-tree: static\end{tabular}} &
  \textbf{Header only} \\ \hline
\textbf{FLANN} &
  \textbf{\begin{tabular}[c]{@{}l@{}}Multi-k-d tree index\\ k-means tree\end{tabular}} &
  \textbf{KNN, AKNN} &
  \textbf{\begin{tabular}[c]{@{}l@{}}Dynamic, self-balancing\end{tabular}} &
  \textbf{} \\ \hline
\textbf{KDTREE1} &
  \textbf{} &
  \textbf{Nearest neighbor} &
  \textbf{Static} &
  \textbf{} \\ \hline
\textbf{KDTREE2} &
  \textbf{} &
  \textbf{KNN} &
  \textbf{Static} &
  \textbf{} \\ \hline
\textbf{KDTREE3} &
  \textbf{} &
  \textbf{KNN} &
  \textbf{Both supported} &
  \textbf{\begin{tabular}[c]{@{}l@{}}Based on nanoflann\\ Header only\end{tabular}} \\ \hline
\textbf{KDTREE4} &
  \textbf{} &
  \textbf{Nearest neighbor} &
  \textbf{\begin{tabular}[c]{@{}l@{}}Dynamic (no deletion), \\ not self-balancing\end{tabular}} &
  \textbf{} \\ \hline
\textbf{libkdtree++} &
  \textbf{} &
  \textbf{\begin{tabular}[c]{@{}l@{}}NN, NN w. range\\ Range (cubic)\end{tabular}} &
  \textbf{\begin{tabular}[c]{@{}l@{}}Dynamic, \\ not self-balancing\end{tabular}} &
  \textbf{Header only} \\ \hline
\textbf{libkdtree2} &
  \textbf{} &
  \textbf{\begin{tabular}[c]{@{}l@{}}Nearest neighbor, KNN\\ Range (sphere)\end{tabular}} &
  \textbf{Static} &
  \textbf{} \\ \hline
\textbf{libnabo} &
  \textbf{} &
  \textbf{KNN, KNN w. range} &
  \textbf{Static} &
  \textbf{\begin{tabular}[c]{@{}l@{}}Designed for low \\ dimensional data\end{tabular}} \\ \hline
\textbf{libpatialindex} &
  \textbf{\begin{tabular}[c]{@{}l@{}}MVR/PPR tree \\ TPR tree\end{tabular}} &
  \textbf{KNN} &
  \textbf{\begin{tabular}[c]{@{}l@{}}Dyamic, self-balancing\\ Packing algorithm\end{tabular}} &
  \textbf{} \\ \hline
\textbf{nanoflann} &
  \textbf{} &
  \textbf{KNN} &
  \textbf{\begin{tabular}[c]{@{}l@{}}Both. Dynamic\\ not self-balancing\end{tabular}} &
  \textbf{\begin{tabular}[c]{@{}l@{}}Header only\\ Fork of FLANN\end{tabular}} \\ \hline
\textbf{octree} &
  \textbf{} &
  \textbf{\begin{tabular}[c]{@{}l@{}}NN w. or w/o min distance\end{tabular}} &
  \textbf{Static} &
  \textbf{} \\ \hline
\textbf{PCL} &
  \textbf{} &
  \textbf{\begin{tabular}[c]{@{}l@{}}k-d tree: KNN\\ octree:  KNN, KNN w. radius, ANN;\\ Range (sphere);\\ voxel search, ray intersection\end{tabular}} &
  \textbf{\begin{tabular}[c]{@{}l@{}}k-d tree: static\\ \\ octree: dynamic, \\ self-balancing\end{tabular}} &
  \textbf{} \\ \hline
\textbf{Pico tree} &
  \textbf{} &
  \textbf{\begin{tabular}[c]{@{}l@{}}KNN, ANN, Range (sphere)\end{tabular}} &
  \textbf{Static} &
  \textbf{Header only} \\ \hline
\textbf{R-tree} &
  \textbf{} &
  \textbf{} &
  \textbf{Dynamic, self-balancing} &
  \textbf{Header only} \\ \hline
\textbf{spatial} &
  \textbf{} &
  \textbf{\begin{tabular}[c]{@{}l@{}}Farthest neighbor\\ NN w. or w/o min distance\end{tabular}} &
  \textbf{\begin{tabular}[c]{@{}l@{}}Dynamic trees, can choose \\ if it self-balances\end{tabular}} &
  \textbf{Header only} \\ \hline
\end{tabular}
\vspace{-0.3in}
\end{table}
